# Supplementary material for: Thermodynamic Signatures of Reasoning: Free-Energy and Spectral-Form-Factor Diagnostics for Hallucination Detection in Large Language Models
Source: arXiv:2606.19404 source file (2026-06-17)
Supplement: Supplementary file 1 [file A_proofs_.tex]

\section{Full Proofs}
\label{app:proofs}

\subsection{Proof of Theorem~\ref{thm:lipschitz} (Lipschitz stability)}
\label{app:proof:lipschitz}

\paragraph{Statement.}
Let $L, L' \in \R^{n\times n}$ be symmetric PSD matrices with
$\|L - L'\|_\mathrm{op} \le \varepsilon$.
For every $\beta > 0$ and $t \ge 0$,
\begin{equation*}
|F(\beta) - F'(\beta)| \le \varepsilon, \qquad |g(t) - g'(t)| \le 2 t \varepsilon.
\end{equation*}

\paragraph{Step 1: eigenvalue perturbation.}
Let $\lambda = (\lambda_1, \ldots, \lambda_n)$ and $\lambda' = (\lambda'_1, \ldots, \lambda'_n)$
denote the sorted eigenvalues of $L$ and $L'$. By the Hoffman-Wielandt inequality
\citep{hoffman1953variation},
\begin{equation}
\|\lambda - \lambda'\|_2 \le \|L - L'\|_F \le \sqrt{n}\,\|L - L'\|_\mathrm{op} \le \sqrt{n}\,\varepsilon,
\end{equation}
and in particular 

$\max_k |\lambda_k - \lambda'_k| \le \|L - L'\|_\mathrm{op} \le \varepsilon$.

\paragraph{Step 2: free energy as a 1-Lipschitz function.}
As a function of $\lambda$, the free energy is
\begin{equation*}
F(\beta, \lambda) = -\tfrac{1}{\beta}\log \sum_k e^{-\beta \lambda_k}.
\end{equation*}
Its partial derivative is
\begin{equation}
\begin{aligned}
\tfrac{\partial F}{\partial \lambda_k} = -\tfrac{1}{\beta} \cdot \tfrac{-\beta\, e^{-\beta\lambda_k}}{Z(\beta)}
= p_k(\beta), \\ \quad p_k = \tfrac{e^{-\beta\lambda_k}}{Z(\beta)} \in [0,1].
\end{aligned}
\end{equation}
Since $\sum_k p_k = 1$, $\nabla_\lambda F$ lies in the probability simplex.
Therefore $F$ is $1$-Lipschitz in the $\ell^\infty$ norm:
% \begin{equation*}
% |F(\beta, \lambda) - F(\beta, \lambda')| \le \|\nabla F\|_1 \cdot \|\lambda - \lambda'\|_\infty \le 1 \cdot \varepsilon = \varepsilon.
% \end{equation*}
\begin{equation}
\begin{aligned}
\left|
F(\beta,\boldsymbol{\lambda})
-
F(\beta,\boldsymbol{\lambda}')
\right|
&\leq
\left\|
\nabla_{\boldsymbol{\lambda}} F
\right\|_1
\,
\left\|
\boldsymbol{\lambda}
-
\boldsymbol{\lambda}'
\right\|_\infty \\
&\leq
1 \cdot \varepsilon = \varepsilon .
\end{aligned}
\label{eq:free_energy_lipschitz}
\end{equation}
\paragraph{Step 3: spectral form factor.}
We have $S(t, \lambda) = \sum_k e^{-it\lambda_k}$, so $g(t) = |S|^2/n^2$. Then
% \begin{equation*}
% |S(t, \lambda) - S(t, \lambda')| \le \sum_k |e^{-it\lambda_k} - e^{-it\lambda'_k}| \le \sum_k t \cdot |\lambda_k - \lambda'_k| \le n t \varepsilon,
% \end{equation*}
\begin{align*}
|S(t, \lambda) - S(t, \lambda')|
  &\le \sum_k |e^{-it\lambda_k} - e^{-it\lambda'_k}| \\
  &\le \sum_k t \cdot |\lambda_k - \lambda'_k| \\
  &\le n t \varepsilon.
\end{align*}
using $|e^{ia} - e^{ib}| \le |a - b|$.
Also $|S(t, \lambda)| \le n$ and similarly $|S(t, \lambda')| \le n$. Therefore
% \begin{equation*}
% |g - g'| = \tfrac{1}{n^2}\bigl||S|^2 - |S'|^2\bigr|
% = \tfrac{1}{n^2}|S - S'|\,|S + S'|
% \le \tfrac{1}{n^2} \cdot n t \varepsilon \cdot 2 n
% = 2 t \varepsilon.
% \end{equation*}

\begin{equation}
\begin{aligned}
|g - g'|
&=
\frac{1}{n^2}
\bigl|
|S|^2 - |S'|^2
\bigr| \\
&\leq
\frac{1}{n^2}
|S-S'|
\left(
|S| + |S'|
\right) \\
&\leq
\frac{1}{n^2}
\cdot n t \varepsilon
\cdot 2n \\
&=
2t\varepsilon .
\end{aligned}
\label{eq:sff_stability_bound}
\end{equation}
\hfill$\Box$
\paragraph{Remark (Tightness).}
The bound $|F - F'| \le \varepsilon$ is tight up to a constant: choosing
$L' = L + \varepsilon I$ shifts every eigenvalue by exactly $\varepsilon$, so $F'(\beta) = F(\beta) - \varepsilon$ (since $F$ shifts with a uniform additive constant on eigenvalues). The SFF bound is tight as $\beta \to 0$ for unit-spread spectra.

\subsection{Proof of Theorem~\ref{thm:subsumption} (Strict subsumption)}
\label{app:proof:subsumption}

\subsubsection*{(a) Moment recovery via partition-function derivatives.}
\paragraph{Lemma.}
For all $k \ge 0$,
$M_k(L) = \tfrac{1}{n}\Tr(L^k) = (-1)^k \cdot \tfrac{d^k Z(\beta)}{d\beta^k}\big|_{\beta=0} \big/ n$.

\paragraph{Proof.}
Expand $Z(\beta) = \sum_j e^{-\beta\lambda_j}$ in a Taylor series around $\beta = 0$:
\begin{equation}
\begin{aligned}
Z(\beta)
&=
\sum_j
\sum_{k=0}^{\infty}
\frac{(-\beta)^k \lambda_j^k}{k!}
=
\sum_{k=0}^{\infty}
\frac{(-\beta)^k}{k!}
\sum_j \lambda_j^k
\\
&=
\sum_{k=0}^{\infty}
\frac{(-\beta)^k}{k!}
\operatorname{Tr}(L^k).
\end{aligned}
\label{eq:partition_moment_expansion}
\end{equation}
% \begin{equation}
% Z(\beta) = \sum_j \sum_{k=0}^\infty \frac{(-\beta)^k \lambda_j^k}{k!}
%         = \sum_{k=0}^\infty \frac{(-\beta)^k}{k!} \sum_j \lambda_j^k
%         = \sum_{k=0}^\infty \frac{(-\beta)^k}{k!} \Tr(L^k).
% \end{equation}

Differentiating $k$ times and evaluating at $0$ gives $\tfrac{d^k Z}{d\beta^k}\big|_0 = (-1)^k \Tr(L^k)$,
and dividing by $n$ yields the claim. \hfill$\Box$

\paragraph{Operational recovery.}
With a finite grid $\beta_0 = 0 < \beta_1 < \cdots < \beta_K$ at uniform spacing $h$, the
$k$-th forward finite difference at $0$ approximates $d^k Z / d\beta^k|_0$ to
error $\mathcal{O}(h)$ (or $\mathcal{O}(h^2)$ with central differences if symmetric stencils
are allowed). Newton's identities then convert the power sums $\{M_k\}$ to elementary
symmetric polynomials $\{e_k\}$:
\begin{equation}
\begin{aligned}
k e_k
&=
\sum_{i=1}^{k}
(-1)^{i-1}
e_{k-i}\, p_i, \\
e_0
&=
1, \quad p_i = n M_i(L).
\end{aligned}
\label{eq:newton_identities}
\end{equation}
% \begin{equation}
% k\,e_k = \sum_{i=1}^k (-1)^{i-1} e_{k-i}\, p_i, \quad e_0 = 1, \quad p_i = n M_i(L).
% \end{equation}
The companion polynomial $x^K - e_1 x^{K-1} + e_2 x^{K-2} - \cdots + (-1)^K e_K = 0$
has roots equal to the top-$K$ eigenvalues, which are the \textsc{LapEigvals} features of
\citet{binkowski2025lapeigvals}.

\subsubsection*{(b) Fiedler value as a low-temperature limit.}
For a connected Laplacian $L$, $\lambda_0 = 0$ is the unique smallest eigenvalue, so
% \begin{equation*}
% Z(\beta) - 1 = e^{-\beta\lambda_0} + \sum_{k\ge 1} e^{-\beta\lambda_k} - 1
% = \sum_{k\ge 1} e^{-\beta\lambda_k}
% = e^{-\beta\lambda_1}\bigl(1 + \sum_{k\ge 2} e^{-\beta(\lambda_k - \lambda_1)}\bigr).
% \end{equation*}
\begin{equation}
\begin{aligned}
Z(\beta) - 1
&= \sum_{k\ge 1} e^{-\beta\lambda_k} \\
&= e^{-\beta\lambda_1}
\left(
1 + \sum_{k\ge 2}
e^{-\beta(\lambda_k - \lambda_1)}
\right).
\end{aligned}
\label{eq:partition_gap}
\end{equation}
As $\beta \to \infty$, the bracketed factor $\to 1$ if $\lambda_2 > \lambda_1$
(which holds generically). Taking $-\log$ and dividing by $\beta$:
\begin{equation*}
-\tfrac{1}{\beta}\log(Z(\beta) - 1)
\to \lambda_1, \quad \beta \to \infty.
\end{equation*}
\hfill$\Box$

\subsubsection*{(c) HFER as a spectral truncation.}
With cutoff $\lambda^*$,
$\mathrm{HFER}(\lambda^*) = \sum_{k: \lambda_k > \lambda^*} \lambda_k^2 \,\big/\, \sum_k \lambda_k^2
= M_2 - M_2^{\le \lambda^*}$ where $M_2^{\le \lambda^*} = \tfrac{1}{n}\sum_{k: \lambda_k \le \lambda^*} \lambda_k^2$
is a censored moment. Censored moments are smooth functionals of the spectral density, which is itself reconstructible from sufficiently many partition-function evaluations (Stone-Weierstrass on $[0, \lambda_{\max}]$). \hfill$\Box$

\subsubsection*{Corollary~\ref{cor:dominance} (operational).}
Any prior classifier $f: \mathcal{F}_\mathrm{Bin} \to [0,1]$ (top-$K$ eigenvalues) extends to $\tilde f: \R^{L(3m+p)} \to [0,1]$ by composing with the recovery functional from (a). The AUROC of $\tilde f$ equals the AUROC of $f$ exactly (the composition is
a bijection between input feature spaces); hence the supremum over classifiers on $\Phi$ is at least the supremum over classifiers on $\mathcal{F}_\mathrm{Bin}$. The same argument with (b)+(c) applies to $\mathcal{F}_\mathrm{GoR}$. \hfill$\Box$

\subsection{Proof of Theorem~\ref{thm:pac} (Detection concentration)}
\label{app:proof:pac}

\paragraph{Setup.}
Let $X^+_1, \ldots, X^+_{n_+} \stackrel{i.i.d.}{\sim} P^+$ and $X^-_1, \ldots, X^-_{n_-} \stackrel{i.i.d.}{\sim} P^-$.
The empirical AUROC of the score $\mathcal{D}$ is
\begin{equation*}
\widehat{\mathrm{AUROC}} = \frac{1}{n_+ n_-} \sum_{i=1}^{n_+} \sum_{j=1}^{n_-} \mathbf{1}\bigl[\mathcal{D}(X^-_j) > \mathcal{D}(X^+_i)\bigr],
\end{equation*}
which is a two-sample U-statistic of degree $(1,1)$ over the kernel
$h(X^+, X^-) = \mathbf{1}[\mathcal{D}(X^-) > \mathcal{D}(X^+)] \in \{0,1\}$.

\paragraph{Step 1: lower-bound the population AUROC.}
By Markov's inequality, for any threshold $\tau$ in the range of $\mathcal{D}$,
\begin{equation}
\begin{aligned}
\Delta_\tau
&=
\Pr\!\left[\mathcal{D}(X^-) > \tau\right]
-
\Pr\!\left[\mathcal{D}(X^+) > \tau\right] \\
&=
\int_{\Omega}
\Bigl(
\mathbf{1}\{\mathcal{D}(X^-)>\tau\}
-
\mathbf{1}\{\mathcal{D}(X^+)>\tau\}
\Bigr)
\,dP .
\end{aligned}
\label{eq:deviation_probability_gap}
\end{equation}
% \begin{equation*}
% \Pr[\mathcal{D}(X^-) > \tau] - \Pr[\mathcal{D}(X^+) > \tau] = \int (\mathbf{1}_{>\tau}(d^-) - \mathbf{1}_{>\tau}(d^+)) \, dP,
% \end{equation*}

and integrating against the joint of $(d^+, d^-)$ yields the U-statistic mean. A standard argument (e.g., \citealp[Lemma~A.3]{hand2001simple}) gives
$\E[h] \ge \tfrac{1}{2} + \tfrac{|\Delta|}{2 D_{\max}}$ whenever
$|\mathcal{D}| \le D_{\max}$ and $\Delta = \E[\mathcal{D}(X^-)] - \E[\mathcal{D}(X^+)] > 0$.

\paragraph{Step 2: concentration via U-statistic Hoeffding.}
The two-sample U-statistic $\widehat{\mathrm{AUROC}}$ is bounded in $[0,1]$, so by
Hoeffding's inequality for two-sample U-statistics
\citep[Thm.~7.1]{hoeffding1963probability}:
% \begin{equation}
% \Pr\Bigl[\,|\widehat{\mathrm{AUROC}} - \E[\widehat{\mathrm{AUROC}}]| > u\,\Bigr] \le 2 \exp(-2 n_\mathrm{eff} u^2),
% \end{equation}
\begin{equation}
\begin{aligned}
\Pr\Bigl[
\bigl|
\widehat{\mathrm{AUC}}
-
\mathbb{E}[\widehat{\mathrm{AUC}}]
\bigr|
> u
\Bigr]
&\leq
2\exp\left(
-2 n_{\mathrm{eff}} u^2
\right).
\end{aligned}
\label{eq:auroc_concentration}
\end{equation}

where $n_\mathrm{eff} = \min(n_+, n_-)$.
Setting the RHS equal to $\delta$ yields $u = \sqrt{\log(2/\delta)/(2 n_\mathrm{eff})}$.

\paragraph{Step 3: combine.}
With probability at least $1 - \delta$,
$\widehat{\mathrm{AUROC}} \ge \E[\widehat{\mathrm{AUROC}}] - u \ge \tfrac{1}{2} + \tfrac{|\Delta|}{2 D_{\max}} - u$.
Note the empirical AUROC is itself the U-statistic, which is what we measure; the bound \eqref{eq:pac} thus holds. \hfill$\Box$

\paragraph{Remark.}
The bound is loose by a constant factor: a tighter analysis using the DKW-type results for empirical distribution functions gives
$\sqrt{\log(2/\delta)/n_\mathrm{eff}}$ at the cost of additional assumptions on the score density. We use Hoeffding for transparency.
