# Supplementary material for: Thermodynamic Signatures of Reasoning: Free-Energy and Spectral-Form-Factor Diagnostics for Hallucination Detection in Large Language Models
Source: arXiv:2606.19404 source file (2026-06-17)
Supplement: Supplementary file 2 [file B_unfolding_.tex]

\section{Unfolded Spectrum and the GOE Reference}
\label{app:unfolding}

The random-matrix-theory predictions invoked in
Sections~\ref{sec:method:sff}--\ref{sec:exp:rmt} are statements about the \emph{level statistics} of the unfolded spectrum, not the raw spectrum. This appendix gives the standard derivation and our concrete unfolding procedure.

\subsection{Why unfold?}
For two systems with different mean spectral densities, raw eigenvalues are not comparable: a scale change in $L$ rescales $\{\lambda_k\}$ uniformly without changing local correlations. Unfolding removes this trivial scale.

\paragraph{Procedure.}
Sort the eigenvalues $\lambda_0 < \lambda_1 < \cdots < \lambda_{n-1}$ and let $N(\lambda) = |\{k : \lambda_k \le \lambda\}|$ be the staircase counting function. We fit a degree-$5$ polynomial $\bar N(\lambda)$ to the bulk of $N(\lambda)$, excluding the trivial zero mode and the top $5\%$ of eigenvalues to avoid edge effects. The unfolded eigenvalues are 
\begin{equation*}
\hat\lambda_k = \bar N(\lambda_k).
\end{equation*}
By construction the local mean spacing of $\{\hat\lambda_k\}$ is
approximately $1$ in the bulk. All main-text results use this polynomial
unfolding.

\paragraph{Linear sanity check.}
For approximately uniform spectra, the simpler linear rescaling
\begin{equation*}
\tilde\lambda_k = (\lambda_k - \lambda_0) / \bar s,
\qquad
\bar s = (\lambda_{n-1} - \lambda_0)/(n-1),
\end{equation*}
agrees with our polynomial unfolding when $\mu_\ell$ is close to uniform. We use it only as a sanity check on our pipeline; it produces $\langle r \rangle$ statistics within $0.6\%$ of the polynomial scheme on both synthetic GOE / Poisson controls and on real LLM spectra.

\paragraph{Sensitivity to degree.}
We re-ran the spacing-ratio detector with polynomial degrees $\{3, 5, 7, 9\}$. The resulting $\langle r \rangle$ statistics differed by less than $0.4\%$ on synthetic controls, and the AUROC of the unsupervised detector on HaluEval differed by less than $0.6$ AUROC points across the four choices. Conclusions are not sensitive to the unfolding-degree
choice within this range.

\subsection{Connected GOE spectral form factor}
\label{app:KGOE}
The Gaussian Orthogonal Ensemble (GOE) on real symmetric $n \times n$ matrices yields, in the large-$n$ limit with unit mean spacing, the analytic \emph{connected} spectral form factor \citep[Eq.~6.2.27]{mehta2004random}:
\begin{equation}
K_\GOE(\tau) =
\begin{cases}
2\tau - \tau \log(1 + 2\tau) & 0 \le \tau \le 1, \\[2pt]
2 - \tau \log\!\Bigl(\dfrac{2\tau+1}{2\tau-1}\Bigr) & \tau > 1,
\end{cases}
\label{eq:KGOE}
\end{equation}
where $\tau = t/(2\pi)$. The curve exhibits the universal \emph{dip}-\emph{ramp}-\emph{plateau} structure:
\begin{itemize}\itemsep1pt\topsep1pt 
\item $K_\GOE(0) = 0$ (the dip), where level repulsion suppresses
  high-frequency Fourier components;
\item linear ramp on $[0, 1]$ from $0$ to $K_\GOE(1) = 2 - \log 3
  \approx 0.901$;
\item plateau $K_\GOE(\tau) \to 1$ as $\tau \to \infty$
  (since $\tau \log\!\bigl(\tfrac{2\tau+1}{2\tau-1}\bigr) \to 1$).
\end{itemize}
For a Poisson process of eigenvalues (no level repulsion), $K_\mathrm{Poisson}(\tau) = 0$ at small $\tau$ in the connected
convention a flat absence of ramp. The dip-ramp-plateau versus flat distinction is the empirical RMT signal we exploit.

\paragraph{Connected convention.}
The form factor used throughout this paper and in Eq.~\eqref{eq:devscore} is the \emph{connected} SFF (defined in Eq.~\eqref{eq:sff-connected} of the main text), in which the ensemble-disconnected piece is subtracted. With this convention,
$g_\ell^\mathrm{conn}(t) \in [0,1]$ and $K_\GOE(\tau) \in [0,1]$, so the integrand of $\mathcal{D}(x)$ is bounded by $1$ and $D_{\max} = T$ as stated in \S\ref{sec:method:detector}.

\subsection{Spacing-ratio statistic}
A complementary level-statistic detector, introduced by \citet{atas2013distribution}, avoids unfolding entirely. Define
$s_i = \lambda_{i+1} - \lambda_i$ and the consecutive ratio $r_i = \min(s_i, s_{i+1})/\max(s_i, s_{i+1}) \in [0,1]$. The mean ratio
admits closed-form predictions:
\begin{equation}
\begin{aligned}
\langle r \rangle_\mathrm{Poisson}
  &= 2\log 2 - 1 \approx 0.3863, \\
\langle r \rangle_\GOE
  &= 4 - 2\sqrt{3} \approx 0.5359.
\end{aligned}
\label{eq:gap_ratio_reference_values}
\end{equation}
We empirically obtain $\langle r \rangle \approx 0.531$ on synthetic GOE samples and $\langle r \rangle \approx 0.387$ on Poisson samples ($n = 64$, $500$ samples each), within $1\%$ of theory.
